# Supplementary material for: Chasing the Tail in Monocular 3D Human Reconstruction with Prototype Memory
Source: arXiv:2012.14739 source file (2020-12-29)
Supplement: Supplementary file 1 [file supplementary.tex]

\section{Implementation Details}
\label{sec:appendix}
